# Supplementary material for: MoCoLSK: Modality Conditioned High-Resolution Downscaling for Land Surface Temperature
Source: arXiv:2409.19835 source file (2025-03-02)
Supplement: Supplementary file 1 [file 9-appendix.tex]

% \appendices
% \section{HeiheLST DATASET AND GrokLST TOOLKIT}
% \subsection{Acquisition times of selected images in HeiheLST}
% Appendix one text goes here.
